# Supplementary material for: Marlin: Efficient Coordination for Autoscaling Cloud DBMS (Extended Version)
Source: arXiv:2508.01931 source file (2025-08-03)
Supplement: Supplementary file 1 [file MarlinAppendix.pdf]

The following is supplementary material attached as an appendix.

## A Proof of the Correctness Invariants

We provide a proof of Marlin's correctness invariants. We start with a serializability guarantee, leading to three small invariants that together compose the core Exclusive Granule Ownership invariant. Then, correctness of user transactions naturally follows.

We start by defining the **owner** of a granule  $G$  as a node  $N$  where: (D1)

$$N.GTable[G].NodeID == N$$

**I0: Reconfiguration Transactions are Serializable.** For any log instance (a GLog or the SysLog), *MarlinCommit* ensures that all reconfiguration transactions on the log are serialized.

*PROOF.* All transactions end with *MarlinCommit*, which involves the *TryLog* compare-and-swap operation that we assume is supported atomically by the storage service. For any log, the input to the compare-and-swap is a tracked LSN that is only updated by the last *TryLog* operation itself.

This implies that, throughout the lifetime of any committed reconfiguration transaction (or more generally, throughout the time span starting from the last completion of any transaction up to the completion of the committed one), no other transactions touching the same log could have been committed. By contradiction, all transactions involving the log are serialized in the same order as the completed *TryLogs*.  $\square$

Given this result I0, if some invariant holds for each individual transaction in isolation, then by induction (on the serialized order of transactions), it also holds for Marlin in general.

**I1: Nodes and GTables are One-One Mapped.** Membership is dictated by the SysLog and is always kept well-formed. To be more specific, nodes always join the cluster or get removed from the cluster in discrete granularity.

*PROOF.* We enumerate over reconfiguration transaction types that involve the SysLog.

AddNodeTxn: Exactly one node is added and associated with a new, unique GTable.

DeleteNodeTxn: Exactly one node is removed along with its GTable/GLog partition.

Other transactions: Never update membership.  $\square$

**I2: Every Granule Has At Least One Owner.** For each granule, there exists at least one owner node of it.

*PROOF.* We enumerate over reconfiguration transaction types that involve GTable update(s).

MigrationTxn: At commit, we have  $dst.GTable[G].NodeID == dst$ , meaning that  $dst$  is an owner of  $G$ .

RecoveryMigrTxn: At commit,  $dst$  is an owner of  $G$  following the same reasoning as above.  
Other transactions: Never update GTables.  $\square$

**I3: Every Granule Has At Most One Owner.** For each granule, there exists at most one owner node of it.

*PROOF.* We enumerate over reconfiguration transaction types that involve GTable update(s).

MigrationTxn: We use induction. At a base state without any migrations, this invariant obviously holds.

Now, assume it holds at the start of a successful *MigrationTxn*. Because  $src.GTable[G].NodeID == src$  is required in order for the transaction to commit,  $src$  is an owner of  $G$  at the start. Therefore,  $src$  is the only owner at the start.

RecoveryMigrTxn: We use induction similarly. Base state obviously holds, and that every transaction exactly swaps the owner of  $G$  from  $src$  to  $dst$ . Therefore,  $dst$  is the only owner at the end.

☐☐☐

---

MODULE *Marlin*

EXTENDS *FiniteSets, Sequences, Integers, TLC*

---

Model inputs & assumptions.

CONSTANT *Nodes*,           set of all compute nodes  
           *Granules*,        set of all data granules  
           *NumMigrations*   number of migrations to run

$NodesAssumption \triangleq \wedge IsFiniteSet(Nodes)$   
                                    $\wedge Cardinality(Nodes) \geq 1$

$GranulesAssumption \triangleq \wedge IsFiniteSet(Granules)$   
                                    $\wedge Cardinality(Granules) \geq Cardinality(Nodes)$

$NumMigrationsAssumption \triangleq \wedge NumMigrations \in Nat$   
                                    $\wedge NumMigrations \geq 2$

ASSUME  $\wedge NodesAssumption$   
            $\wedge GranulesAssumption$   
            $\wedge NumMigrationsAssumption$

---

Useful constants & typedefs.

$$\text{Range}(f) \triangleq \{f[x] : x \in \text{DOMAIN } f\}$$

a valid *GTable* is a map from granules to nodes  
 $GTables \triangleq [Granules \rightarrow Nodes]$

$$\text{InitGTable} \triangleq \text{CHOOSE } gtab \in GTables : \text{Range}(gtab) = Nodes$$

a valid *GLog* is a log of *GTable* update actions  
 $Updates \triangleq \{update \in [id : Nat,$   
 $\quad gran : Granules,$   
 $\quad old : Nodes,$   
 $\quad new : Nodes] :$   
 $\quad update.old \neq update.new\}$

$$\text{Update}(i, g, o, n) \triangleq [id \mapsto i, gran \mapsto g, old \mapsto o, new \mapsto n]$$

$$GLogs \triangleq \{log \in Seq(Updates) : Len(log) \leq NumMigrations\}$$

disaggregated storage state: each node maintains its own *Glog*,  
 and materializes it into its own view of *GTable*  
 $Storages \triangleq [glogs : [Nodes \rightarrow GLogs],$   
 $\quad gtabs : [Nodes \rightarrow GTables]]$

$$\text{InitStorage} \triangleq [glogs \mapsto [n \in Nodes \mapsto \langle \rangle],$$
  
 $\quad gtabs \mapsto [n \in Nodes \mapsto \text{InitGTable}]]$ 

Main algorithm in *PlusCal*.

**algorithm** *Marlin*

**variable**  $storage = \text{InitStorage},$     disaggregated storage state  
 $nextUpdateId = 0,$     randomly unique *updateIds*  
 $numDone = 0$     number of migrations done

**define**

$$\text{IsNewUpdate}(n, u) \triangleq u.id \notin \{v.id : v \in \text{Range}(storage.glogs[n])\}$$

consider execution terminated when all migrations have been done and  
 all nodes' *GTables* are the same  
 $terminated \triangleq$   
 $\quad \wedge numDone = NumMigrations$   
 $\quad \wedge \text{Cardinality}(\text{Range}(storage.gtabs)) = 1$

**end define ;**

Node picks a granule and a peer to do a migration push.

This is the “*MigrationTxn*” that happens proactively between src and dst  
 where src is the old owner and dst is the new owner.

**macro** *DoMigrate*(*n*)**begin**

**await**  $numDone < NumMigrations ;$

**with**  $g \in Granules,$   
 $p \in \{p \in Nodes : p \neq n\}$

**do**

a migration txn first checks that on both source and target, their  
*GTables* both say that *k* is assigned to the source right now

**await**  $\wedge storage.gtabs[n][g] = n$   
 $\quad \wedge storage.gtabs[p][g] = n ;$

append to both source and target *GLogs* to assign *g* to the target

```

    storage.glogs[n] := Append(@, Update(nextUpdateId, g, n, p)) ||
    storage.glogs[p] := Append(@, Update(nextUpdateId, g, n, p)) ||
    materialize into their GTables
    storage.gtabs[n][g] := p ||
    storage.gtabs[p][g] := p ;
  end with ;
  nextUpdateId := nextUpdateId + 1 ;   in practice, this is say a random hash
  numDone := numDone + 1 ;
end macro ;

```

Node receives gossiping of an update action from some peer (or probes the *log* of some peer and finds a difference; both ways are mathematically equivalent). This is part of the “*MetaRefresh*” that non-owners do to keep state up-to-date.

```

macro DoRefresh(n) begin
  with p ∈ {p ∈ Nodes : p ≠ n},
    u ∈ Range(storage.glogs[p])
  do
    this update action is not in my GLog yet, and that the old holder
    of the updated granule matches what's in my GTable
    await ∧ IsNewUpdate(n, u)
      ∧ storage.gtabs[n][u.gran] = u.old ;
    append it to my GLog and update my GTable view
    storage.glogs[n] := Append(@, u) ||
    storage.gtabs[n][u.gran] := u.new ;
  end with ;
end macro ;

```

Compute node main loop.

```

process Node ∈ Nodes
begin
  nloop: while ¬terminated do
    either
      DoMigrate(self) ;
    or
      DoRefresh(self) ;
    end either ;
  end while ;
end process ;
end algorithm ;

```

---

#### MODULE Marlin\_MC

---

EXTENDS Marlin

TLC config-related defs.

```

ConditionalPerm(set) ≜ IF Cardinality(set) > 1
  THEN Permutations(set)
  ELSE {}

```

```

SymmetricPerms ≜ ConditionalPerm(Nodes)
                ∪ ConditionalPerm(Granules)

```

```

ConstNumMigrations ≜ 6

```

---

Type check invariant.

$$\begin{aligned} TypeOK &\triangleq \wedge storage \in Storages \\ &\quad \wedge numDone \geq 0 \\ &\quad \wedge numDone \leq ConstNumMigrations \end{aligned}$$

THEOREM  $Spec \Rightarrow \Box TypeOK$

NoDualOwnership invariant.

$$PairsOfNodes \triangleq \{pn \in \text{SUBSET } Nodes : Cardinality(pn) = 2\}$$

$$\begin{aligned} NoDualOwnership &\triangleq \\ &\quad \forall g \in Granules : \\ &\quad \quad \forall pn \in PairsOfNodes : \\ &\quad \quad \quad \text{LET } n1 \triangleq \text{CHOOSE } n \in pn : \text{TRUE} \\ &\quad \quad \quad \text{IN } \text{LET } n2 \triangleq \text{CHOOSE } n \in pn : n \neq n1 \\ &\quad \quad \quad \quad \text{IN } \neg(\wedge storage.gtabs[n1][g] = n1 \\ &\quad \quad \quad \quad \quad \wedge storage.gtabs[n2][g] = n2) \end{aligned}$$

THEOREM  $Spec \Rightarrow \Box NoDualOwnership$

HasOneOwnership invariant.

$$\begin{aligned} HasOneOwnership &\triangleq \\ &\quad \forall g \in Granules : \\ &\quad \quad \exists n \in Nodes : \\ &\quad \quad \quad storage.gtabs[n][g] = n \end{aligned}$$

THEOREM  $Spec \Rightarrow \Box HasOneOwnership$

Marlin\_MC.cfg

SPECIFICATION Spec

CONSTANTS

Nodes = {n1, n2, n3}  
Granules = {g1, g2, g3, g4, g5, g6}  
NumMigrations <- ConstNumMigrations

SYMMETRY SymmetricPerms

INVARIANTS

TypeOK  
NoDualOwnership  
HasOneOwnership

CHECK\_DEADLOCK TRUE
